# Supplementary material for: Scalable Neural-Probabilistic Answer Set Programming
Source: arXiv:2306.08397 source file (2023-06-14)
Supplement: Supplementary file 1 [file appendix.tex]

%Accuracy overview
\begin{table}
        \centering
        
        \begin{tabular}{lrrrrrrrrrr}
        \toprule
        Neural &Task & \multicolumn{4}{c}{$\mathit{Shooting^{k}}$}&\multicolumn{4}{c}{$\mathit{Top^{k}}$} & SLASH\\
        
               Model & & k=1 & k=3 & k=5 & k=10 &k=1 & k=3 & k=5 & k=10 &  \\
            \midrule
    NN & T1   & 27.24 & 50.30 & 85.25 & 98.71 & 
           73.08* &98.80 & 98.79 & 98.78 &  98.83 \\
       & T2& 18.73  & 19.91 & 18.74 & 28.23 
       & 98.77 & 98.76 & 98.79 & 98.71 & 98.79\\
       & T3  & 20.63 & 18.80 & 21.70 & 22.41 & 98.72 & 98.68 & 80.85* & 98.75 & 98.89\\
        \midrule
          PC & T1   & 25.02 & 45.84 & 73.78 & 95.32 & 73.71* & 93.05 & 92.85 & 92.02 & 95.32 \\
          & T2 &  16.48 & 17.79 & 16.91 & 25.30 & 82.40 & 86.68 &79.74 & 79.57 & 95.05  \\
          & T3 & 16.81 & 16.88 & 18.00 & 18.15 & 31.21 & 27.18 & 24.20 & 23.83 &  95.23  \\
        \bottomrule
        \end{tabular}

    \caption{Accuracy Comparison between $\mathit{Shooting^{k}}$, $\mathit{Top^{k}}$ within SLASH PC. We compare the method on three different Tasks T1-T3.  sum2(\img{graphs/handwritten_digit_three.svg},\img{graphs/handwritten_digit_seven.svg},10)  sum3(\img{graphs/handwritten_digit_three.svg},\img{graphs/handwritten_digit_seven.svg},\img{graphs/handwritten_digit_five.svg},15) sum4(\img{graphs/handwritten_digit_three.svg},\img{graphs/handwritten_digit_seven.svg},\img{graphs/handwritten_digit_five.svg},\img{graphs/handwritten_digit_two.svg},17)
    }
    \label{tab:shot-and-top-k}
\end{table}
